# Supplementary material for: Algorithm Configuration for Structured Pfaffian Settings
Source: arXiv:2409.04367 source file (2025-05-22)
Supplement: Supplementary file 1 [file additional_applications.tex]

\subsection{Differentiable Neural Architecture Search}

Neural Architecture Search (NAS) \cite{zoph2016neural, pham2018efficient, liu2018progressive} constitutes a research domain focused on the automated discovery and optimization of neural network architectures tailored to specific tasks. Departing from traditional reliance on human domain experts, NAS harnesses the ever-expanding computational capabilities and machine learning methods to autonomously identify more efficient architectures, considering factors like architecture size, training and inference speed, performance on specific tasks, among others.

Common strategies in NAS typically involve the application of evolutionary approaches \cite{liu2021survey} or reinforcement learning techniques \cite{zoph2016neural} across a discrete or non-differentiable architecture search space. This process, however, demands substantial computational resources due to the intricate nature of the search space, making the process of NAS computationally expensive. Addressing this computational challenge, Liu et al. \cite{liu2018darts} made strides by narrowing down the search task to identify the optimal activation function. Their proposal involves incorporating multiple activation functions in each activation node, and learning of weights for each considered activation function. After the search phase, only the activation function with the highest weight is integrated into the final architecture. Though more restrictive, the entire search process is fully differentiable, improving computational tractability compared to previous methodologies.

In this section, we aim to explore the learnability of differential neural architecture search for a simple DNN, under the assumptions that all the considered activation functions are Pfaffian functions. It is important to note that this assumption is very reasonable, given that nearly all commonly used activation functions in machine learning naturally fall into this category.

\subsubsection{Problem Settings}
% \noindent We consider the problem of multivariate parametric regression, where given a dataset $(\boldsymbol{X}, \boldsymbol{Y})$

We consider a feed-forward neural network $f$ with $L$ layers. We denote $W_i$ as the number of parameters in the $i^{th}$ layer, and let $W = \sum_{i=1}^LW_i$. 

In each layer, we have to choose an activation function from a set $\cO = \{o_1, \dots, o_\omega\}$ of various Pfaffian activation functions. For example, common activation functions such as $\tanh$, $\sigmoid$, \dots\ are Pfaffian functions. 

Liu et al. \cite{liu2018darts} proposed a simple way of choosing activation function: at training time, they define a general activation functions $\sigma$ which is the weighted combination of activation functions in $\cO$. In each layer $i \in [L]$, the activation function $o_j$ ($j \in [\omega]$) is assigned with a weight $\alpha_{i, j}$. The combined activation function can be written as
\begin{equation*}
    \begin{aligned}
        \sigma_i(x) = \sum_{j=1}^\omega \frac{e^{\alpha_{i, j}}}{\sum_{t = 1}^{\omega}e^{\alpha_{i, t}}}o_j(x)
    \end{aligned}
\end{equation*}
After the training process, the actual activation function in each node $i$ is chosen by discretizing the combined activation $\sigma_i$ to $\overline{o}_{i} = o_{s_i}$, where
\begin{equation*}
    \begin{aligned}
        s_i = \argmax_{t \in \omega}\alpha_{i, t}.
    \end{aligned}
\end{equation*}

In the parametric regression setting, the output of the final layer corresponds to prediction $f(a,x)=\hat{y}\in\bbR^D$, where $\boldsymbol{a}\in\bbR^{\omega L + W}$ is the vector of parameters, including the architecture hyperparameters $\alpha_{i,j}$ and the network weights. The validation loss on a single validation example $(x,y)$ is given by $||f(a,x)-y||^2$, and on a set of $m$ validation examples as $\ell(a, X,Y)=\frac{1}{m}\sum_{(x,y)\in(X,Y)}||f(a,x)-y||^2$. For a fixed validation dataset $(X,Y)$, the dual class of loss functions is given by $\cL=\{\ell_{(X,Y)}(a):\bbR^{\omega L+W}\rightarrow \bbR^{D}\mid \ell_{(X,Y)}(a)=\ell(a, X,Y), (X,Y)\in (\cX\times\bbR^D)^m \}$. 

\iffalse
\begin{lemma}
    \normalfont{(Layer wise output of Neural Networks with Pfaffian activation functions)} Assume that the output $z_{i-1}$ of layer $(i - 1)^{th}$ corresponding to an input $x \in \cX$ is a $D_{i - 1}$-dimensional vectors, of which each element is a Pfaffian function from the same Pfaffian chain $C_i$ with length $q$ and Pfaffian degree $M$, and of degree at most $\Delta$. We also assume that each activation function $o \in \cO$ is a Pfaffian function from the Pfaffian chain $C_\cO$ with length $q_\cO$ and Pfaffian degree $M_\cO$. Then the output $z_{i}$ of layer $i^{th}$ 
    \begin{equation}
        \begin{aligned}
            z_{i} = \sum_{j=1}^\omega \frac{e^{\alpha_{i, j}}}{\sum_{k = 1}^{\omega}e^{\alpha_{i, k}}}o_j(W_iz_{i - 1})
        \end{aligned}
    \end{equation}
    where $W_i$ is the is a $D_{i}$-dimensional vector, of which each element is a Pfaffian function from the same Pfaffian chain $C_{i}$ with length \blue{TODO} and Pfaffian degree \blue{TODO}.
\end{lemma}
\proof \quad \\ 
Consider $z_{i, j}$  which is the $j^{th}$ element of output vector $z_{i}$. By definition, we can write $z_{i, j}$ as
\begin{equation}
    \begin{aligned}
        z_{i + 1, j} = \sum_{j=1}^\omega \frac{e^{\alpha_{i, j}}}{\sum_{k = 1}^{\omega}e^{\alpha_{i, k}}}o_i(\inner{W_{i, j},z_i})
    \end{aligned}
\end{equation}
where $W_{i, j}$ is the $j^{th}$ row vector of weight matrix $W_{i}$. 

Trivially, $\inner{W_{i, j},z_i}$ is a a Pfaffian function from the same Pfaffian chain $C_i$ with length $q$ and Pfaffian degree $M$, and of degree at most $\Delta$. 
\fi

\begin{theorem} \label{thm:nas-pdim}
     Let $\cL$ denote the dual class validation loss function defined above, and $\cO=\{o_1,\dots,o_{\omega}\}$ denote the set of $\omega$ activation functions, where each activation function $o \in \cO$ is a Pfaffian function from the Pfaffian chain $C_\cO$ with length $q_\cO$ and Pfaffian degree $M_\cO$. Let $L$ denote the number of layers and $W$ denote the total number of neural network weights (both assumed fixed, the architecture search is over the activation functions). Then, 
    $$\Pdim(\cL) = O\left(L^2q_{\cO}^2+(L(q_{\cO}+\omega)+W)\log(LM_{\cO}(\omega+W))+(\omega L+W)\log (\omega L)\right).$$
\end{theorem}

\begin{proof}
    Consider $z_{i, j}$  which is the $j^{th}$ element of output vector $z_{i}$ when computing the validation loss on $(x,y)$. By definition, we can write $z_{i, j}$ as
\begin{equation}
    \begin{aligned}
        z_{i + 1, j} =  o_{s_i}(\inner{W_{i, j},z_i})
    \end{aligned}
\end{equation}
where $W_{i, j}$ is the $j^{th}$ row vector of weight matrix in layer $i$, $z_0=x$. $s_i$ can be determined by computing at most $\omega^2$ distinct predicates $\alpha_{i,t_1}\gtrless \alpha_{i,t_2}$ in a GJ algorithm for each layer $i$, therefore the total number of distinct such predicates is at most $\omega^2L$. 

Further, by the lemma on composition of Pfaffians and an induction on the number of layers $i$, $z_{i,j}$ is a Pfaffian function of chain length at most $i q_{\cO}$, and Pfaffian degree at most $i(M_{\cO}+1)$. Indeed, $z_{i + 1, j} =  o_{s_i}(\inner{W_{i, j},z_i})$ is a composition of $o_{s_i}$ and $\inner{W_{i, j},z_i}$. By inductive hypothesis, $z_i$ is a Pfaffian function of chain length at most $i q_{\cO}$ (and Pfaffian degree at most $i(M_{\cO}+1)$), and therefore so is $\inner{W_{i, j},z_i}$ (with Pfaffian degree at most $i(M_{\cO}+1)+1$). Now  Lemma \ref{lm:composition-pfaffian} implies that $z_{i + 1, j}$ is Pfaffian with chain length at most $i q_{\cO}+q_{\cO}$ and Pfaffian degree at most $i(M_{\cO}+1)+1+M_{\cO}=(i+1)(M_{\cO}+1)$, establishing the inductive claim.

The final predicate computes $\ell(a,X,Y)\gtrless r$ for $r\in\bbR$. By the above argument, this predicate is a Pfaffian function of chain length at most $q=Lq_{\cO}$, Pfaffian degree no more than $M=(L+1)M_{\cO}$ and degree $\Delta=2$. The number of distinct predicates needed to compute the loss using the GJ algorithm is therefore $K=\omega^2 L +1$.

Finally note that we have $d=\omega L + W$ total parameters, and $d':=d+1=\omega L + W+1$. We can now apply Theorem \ref{thm:pfaffian-gj-algorithm} to complete the proof. Indeed we get that

\begin{align*}
    \Pdim(\cL) &\leq q(q - 1) + 2q\log \Delta + 2(2d' + q)\log(\Delta + M) + 2(2q + d')\log(d' + 1) + 2d'\log(2d') + 2d'\log K\\
    &=O\left(q^2+(q+d)\log((\Delta+M)d)+d\log K\right) \\
    &=O\left(L^2q_{\cO}^2+(Lq_{\cO}+L\omega+W)\log((LM_{\cO}+2)(L\omega + W))+(L\omega+W)\log (\omega^2L+1)\right)\\
    &=O\left(L^2q_{\cO}^2+(L(q_{\cO}+\omega)+W)\log(LM_{\cO}(\omega+W))+(\omega L+W)\log (\omega L)\right).
\end{align*}
% \red{I think the number of predicates $K$ here is only 1, since we only have one conditional statement in the last step $\ell(a, X, Y) \gtrless r$.}

\end{proof}

\subsection{Data-driven graph convolutional network with Gaussian kernel}
Graph neural networks (GNN) \cite{zhou2020graph, scarselli2008graph} represent a specialized neural architecture designed for handling data stored in graph structures. The capability of GNN lies in its ability to capture the inherent structure of graphs through the information passing among nodes within the graph. This class of neural network architecture holds significant importance in machine learning, given the prevalence of graph-structured data across diverse domains. 
Specifically, Graph convolutional networks (GCN) \cite{kipf2016semi} have garnered considerable attention within the research community thanks to their state-of-the-art performance and computational efficiency. In this section, our goal is to analyze the learning guarantee of GCN within a simple context. Additionally, we introduce the extra assumption that we also aim to learn the Gaussian Kernel parameter, a crucial factor for distance scaling in graph data.
\subsubsection{Problem setting}
% \red{Current problems: 
% \begin{itemize}
%     \item If we follow the settings from \cite{kipf2016semi}, where we use a simple convolutional neural network which takes an adjacent matrix $A$, and feature matrix $X$, and outputs the logit score of $Z = f(A, X)$ which predicts the class that nodes belong to, we should follows the two layers models for simplicity. However, there are some current problems with this direction:
%     \begin{itemize}
%         \item We might want to incorporate a metric learning parameter
%         \begin{equation*}
%             B_{ij} = \exp\left(-\frac{d(i, j)}{2\alpha^2}\right),
%         \end{equation*}
%         where $i, j \in [n]$ are nodes in the graph, $d(i, j)$ is given, and $\alpha$ is the metric learning parameter. This will makes the problem does not make sense since at each forward time, we have to re-calculate the matrix $\boldB = [B_{ij}]$. However, in the original model, the distance matrix $\boldA = [A_{ij}]$, where $A_{ij} = \exp(-d(i, j))$, is calculated once, which makes it efficient. This means that the problem setting is not well-motivated in this case. $\rightarrow$ we can still do that and ignore the computation inefficiency problem (?)
%     \end{itemize}
%     \item If we follow the settings from \cite{scarselli2018vapnik}, then things will be overlapped with the results of that paper. 
% \end{itemize}
% }

\paragraph{Notation.} Consider a graph $G = (\cV, \cE)$, where $\cV$ and $\cE$ are sets of vertice and edges, respectively. $G$ is associated with data $X$ which is the representation of the nodes. We also have a set of node indices 
 $\cY_L$ of labeled nodes, each of which belongs to one of $F$ labels ($F \in \bbN$), and a corresponding binary matrix $Y $ of size $\abs{\cY_L} \times F$ where the row $Y_l$ corresponds to the label vector of node $l \in \cY_L$. That is, if $Y_l = (0, \dots, 0, 1, 0 \dots, 0)$ is a vector of zero except in the $i^{th}$ coordinate where the value is one, then the node $l$ is of class $i$. 
 
 We want to build a model for classifying the other unlabelled nodes. To do that, we train a graph convolutional network (GCN) \cite{kipf2016semi} using semi-supervised learning. The formal notations and settings are described as follows. 
\begin{itemize}
    \item $A \in \bbR^{n \times n}$ (binary or weighted) is the adjacent matrix of $G$, and let $\tilA = A + I_N$. In this problem, we consider a weighted adjacent matrix w.r.t. Gaussian Kernel $A = [A_{ij}]$ 
    \begin{equation*}
        A_{ij} = \exp(-d(i, j)/2\alpha^2),
    \end{equation*}
    where $d(i, j)$ is the given distance between two nodes $i, j \in \cV$, and $\alpha > 0$ is the tuning parameter.
    \item $X \in \bbR^{n \times d}$ is the given matrix of node feature vector, where $x_i$ for $i \in \cV$ is the $i^{th}$ row of $X$ that represents the feature vector of vertex $i$.
    \item $\tilD$ denotes the degree matrix, where $\tilD_{ii} = \sum_{j}\tilA_{ij}$.
\end{itemize}
Given an adjacent matrix $A$, a feature matrix $X$, and a set of labeled data $Y_L$, we want to train a model that predicts the missing label. 

\paragraph{Network architecture.} We consider a simple two-layer graph convolutional network (GCN) $f$ \cite{kipf2016semi}, which takes the adjacent matrix $A$ and feature matrix $X$ as inputs and outputs $Z = f(X, A)$ of the form 
\begin{equation*}
    \begin{aligned}
        Z = f(X, A) = \text{softmax}(\hat{A}\,\text{ReLU}(\hat{A}XW^{(0)})W^{(1)}),
    \end{aligned}
\end{equation*}
where $\hat{A} = \tilde{D}^{-1/2}\tilde{A}\tilde{D}^{-1/2}$, $W^{(0)} \in \bbR^{d \times d_0}$ is the weight matrix of the first layer, and $W^{(1)} \in \bbR^{d_0 \times F}$ is the hidden-to-output weight matrix. Here, the $z_i$ -- the $i^{th}$ rows of $Z$ -- is the score prediction of the model.
\paragraph{The GCN function class.}
Assuming that we are conducting semi-supervised binary classification. We then evaluate the prediction of the model using binary-cross entropy over all labeled examples 
\begin{equation*}
    \ell_{W, \alpha}(A, X)= - \sum_{l \in \cY_L}\sum_{f=1}^FY_{lf}\log Z_{lf} = - \log\left(\prod_{l \in \cY_L}\prod_{f = 1}^F Z_{lf}^{Y_{lf}}\right),
\end{equation*}
which takes an adjacent matrix $A$ and feature matrix $X$ as inputs, and output a loss value w.r.t the weights $W = (W^{(0)}, W^{(1)})$ of $f$ and the parameter $\alpha$. Consider the GCN function class
\begin{equation*}
    \cF_{\text{GCN}} = \{\ell_{W, \alpha}: \cA \times \cX \rightarrow \bbR \mid W \in \bbR^{d \times d_0} \times \bbR^{d_0 \times F}, \alpha \in (0, \infty)\},
\end{equation*}
where $\cA$ and $\cX$ are the space of valid adjacent matrix and feature matrix, respectively. Our goal now is to give a learning guarantee for the GCN function class $\cF_{\text{GCN}}$. Notice that $-\log(\cdot)$ is a strictly decreasing function, following Lemma \ref{lm:pdim-monotonic-composition}, and the following lemma allows us to simplify the analysis by analyzing a simpler function class. 

\begin{lemma}[\cite{dudle1987universal}]
    \label{lm:pdim-monotonic-composition}
    Suppose $\cF$ is a class of real-valued functions and $\sigma: \bbR \rightarrow \bbR$ is a non-decreasing function. Let $\sigma(\cF)$ denote the class $\{\sigma \circ f: f \in \cF\}$. Then $\Pdim(\sigma(\cF)) \leq \Pdim(\cF)$. The equality holds if $\sigma$ is a continuous and strictly increasing function. 

    On other hand, if $\sigma$ is a non-increasing function then $\Pdim(\sigma(\cF)) \geq \Pdim(\cF)$. The equality holds if $\sigma$ is a continuous and strictly decreasing function.
\end{lemma}

Therefore, we can instead give a learning guarantee by analyzing the pseudo-dimension of a simpler function class $\cF'_{\text{GCN}} = \{\ell'_{W, \alpha}: \cA \times \cX \rightarrow \bbR \mid W \in \bbR^{d \times d_0} \times \bbR^{d_0 \times F}, \alpha \in (0, \infty)\}$, where
\begin{equation*}
     \ell'_{W, \alpha}(A, X) = \prod_{l \in \cY_L}\prod_{f = 1}^F Z_{lf}^{Y_{lf}}.
\end{equation*}

\subsubsection{Analyzing the pseudo-dimension of graph convolutional network} 

We now will derive the pseudo-dimension of $\cF'_{\text{GCN}}$ using Theorem \ref{def:pfaffian-formula}. Given an adjacent matrix $A \in \bbR^{n}$, a feature matrix $X \in \bbR^{n \times d}$, and a threshold $r$, then for any $W$ and $\alpha$, it can be seen that the computation of the boolean statement "$\ell'(A, X; W, \alpha) - r \geq 0$" can be described by Pfaffian GJ algorithm.

\begin{theorem} \label{thm:gcn-pdim}
    Consider the loss function class $\cF'_{\text{GCN}} = \{\ell(\cdot, W, \alpha): \cA \times \cX \rightarrow \bbR \mid W, \alpha\}$ parameterized by $W$ and $\alpha$. Given a problem instance $P = (A, X)$ and a threshold $r$, the computation of the boolean statement "$\ell(A, X; W, \alpha) - r \geq 0$" can be described by a Pfaffian GJ algorithm, of which all the intermediate functions is from the same Pfaffian chain $\cC$ with length at most $n^2 + n + nLFd_0$, predicate complexity at most $Lnd_0$, degree at most $nd_0$. Therefore, $Pdim(\cF'_{\text{GCN}}) = O(n^4w^2).$
\end{theorem}

\proof Recall the computation of $Z$ is defined as: $Z = f(X, A) = \text{softmax}(\hat{A}\,\text{ReLU}(\hat{A}XW^{(0)})W^{(1)})$. We will construct a Pfaffian chain $\cC$ s.t. every element $Z_{ij}$ ($i \in [n]$, $j \in [F]$) is a Pfaffian function from that chains, and bound the total number of distinct functions that element in $Z$ can take. 
\begin{itemize}
    \item First, consider the matrix $\hat{A} = \tilD^{-1/2}\tilA\tilD^{-1/2}$. We have $\hat{A}_{ij} = \tilA_{ij}g_{i}g_{j}$, where 
$$g_{i} = \frac{1}{\sqrt{1 + \sum_{j = 1}^n{\exp(-d(i, j)/2\alpha^2)}}}.$$
Therefore, each $g_i$ ($i \in [n]$) is a Pfaffian function of the chain $\cC(W, \alpha, \frac{1}{\alpha}, A_{11}, \dots, A_{nn}, g_1, \dots, g_{n})$ of $nd_0 + d_0F + 1$ variables and length $n^2 + n$, which implies $\hat{A}_{ij}$ is also a Pfaffian function of the same chain, each of degree at most $3$.

\item Second, consider the matrix $B = \hat{A}XW^{(0)} \in \bbR^{n \times d_0}$. Similarly, we can show that each element of $B$ is a Pfaffian function of chain $\cC$, with degree at most $4$. 

% There are at most $n \times d_0$ distinct functions $B_{ij}$. 

\item Third, consider the matrix $\text{ReLU}(B)$. Now, for each $i, j \in [n] \times [d_0]$, "$B_{ij} \geq 0$" serves as a conditional statement, dictates the form of the next computation. 

\item Fourth, consider the matrix $C = \hat{A}\text{ReLU}(B)W^{(1)} \in \bbR^{n \times F}$. Each element $C_{ij}$ can be computed as
\begin{equation*}
    C_{ij} = \sum_{h = 1}^{d_0}\left(\sum_{k = 1}^{n}\hat{A}_{ik}B_{kh}\bbI(B_{kh} \geq 0)\right)W^{(1)}_{hj}.
\end{equation*}
We can see that each $C_{ij}$ is a Pfaffian function from the same chain $\cC$ with degree at most 6. Besides, there is at most $n \times F \times 2^{n \times d_0}$ such different function $C_{ij}$ can appear.

\item Finally, consider $$\ell'(A, X; W, \alpha) =  \prod_{l \in \cY_L}\prod_{f = 1}^F Z_{lf}^{Y_{lf}} = \prod_{l \in \cY_L}Z_{lf_l^*},$$
where $f_l^*$ is the true class of node $l$, and $Z = \text{softmax}(C) \in \bbR^{n \times F}$, where the softmax operator is applied row-wise. We can also write $\ell'(A, X; W, \alpha)$ more explicitly in terms of $C_{ij}$, for $i, j \in \cY_{L} \times F$ as follow
\begin{equation*}
    \ell'(A, X; W, \alpha) = \prod_{l \in \cY_L}\frac{\exp(C_{lf_l^*})}{\sum_{k = 1}^F\exp(C_{lk})}.
\end{equation*}

WLOG, assume that the given threshold $r > 0$, then the boolean statement "$\ell'(A, X; W, \alpha) - r \geq 0$" has the same truth value as the following boolean statement
\begin{equation}\label{eq:gcn-final}
    \prod_{l \in \cY_L}Z_{lf_l^*} - r \prod_{l \in \cY_L}\left(\sum_{k = 1}^F\exp(C_{lk})\right) \geq 0.
\end{equation}
Now, for all $l$, we add the following function to the Pfaffian chain $\cC$
\begin{equation*}
    \cC \leftarrow \cC \cup \bigcup_{i \in \cY_L, j \in [F]}\{\exp(\hat{A}_{ik}B_{kh}W^{(1)}_{hj}) \mid k \in [d_0], h \in [n]\},
\end{equation*}
which means that the length of $\cC$ now is $n^2 + n + nLFd_0$. Then for any $C_{ij}$, we have
\begin{equation*}
    \exp(C_{ij}) = \prod_{h = 1}^{d_0}\prod_{k  = 1}^n\exp\left(\hat{A}_{ik}B_{kh}\bbI(B_{kh} \geq 0)W^{(1)}_{hj}\right),
\end{equation*}
and in each piece, where the value of $\bbI(B_{kh} \geq 0)$ is determined, $\exp(C_{ij})$ is a Pfaffian function of chain $\cC$ with degree at most $nd_0$. Therefore, the degree of the LHS of \ref{eq:gcn-final} is a Pfaffian function of degree at most $Lnd_0$.
 
\end{itemize}

In summary, the computation of the boolean statement "$\ell'(A, X; W, \alpha) - r \geq 0$" can be described as a Pfaffian GJ algorithm of chain $\cC$ with $w + 1$ variables, length $n^2 + n + nLFd_0$, with predicate complexity of at most $Lnd_0$. Therefore, we conclude that
\begin{equation*}
    \Pdim(\cF'_{GCN}) = O((w + 1)^2(n^2 + n + nLFd_0)^2) = O(n^4w^2).
\end{equation*}
 \qed
